# Supplementary material for: Mining Multi-Label Samples from Single Positive Labels
Source: arXiv:2206.05764 source file (2023-05-28)
Supplement: Supplementary file 1 [file C_Ablation_Study.tex]

\section{Ablation Study}
\label{appendix:ablation_study}

To validate the effects of the temperature $T$ and $\gamma$ in S2M sampling, we perform the ablation study \textbf{CIFAR-10 7to3} and \textbf{CelebA BMS} dataset. In Table~\ref{table:ablation_study}, we report the averaged accuracy and FID of our S2M sampling with different base models; unconditional GANs (GANs), cGAN, and CP-GAN. As expected, with the proper adjustment of hyperparameters, teh accuracy is greatly improved without the degradation of FID. This indicates that our S2M sampling with the proper hyperparameters can sample images within an accurate data space without a trade-off with diversity.

\input{Tables/Table_Ablation_Study}
